# Supplementary material for: DA-VSR: Domain Adaptable Volumetric Super-Resolution For Medical Images
Source: arXiv:2210.05117 source file (2022-10-11)
Supplement: Supplementary file 1 [file SRN_converge.tex]

\begin{figure}[]
    \centering
      \includegraphics[width=1\textwidth]{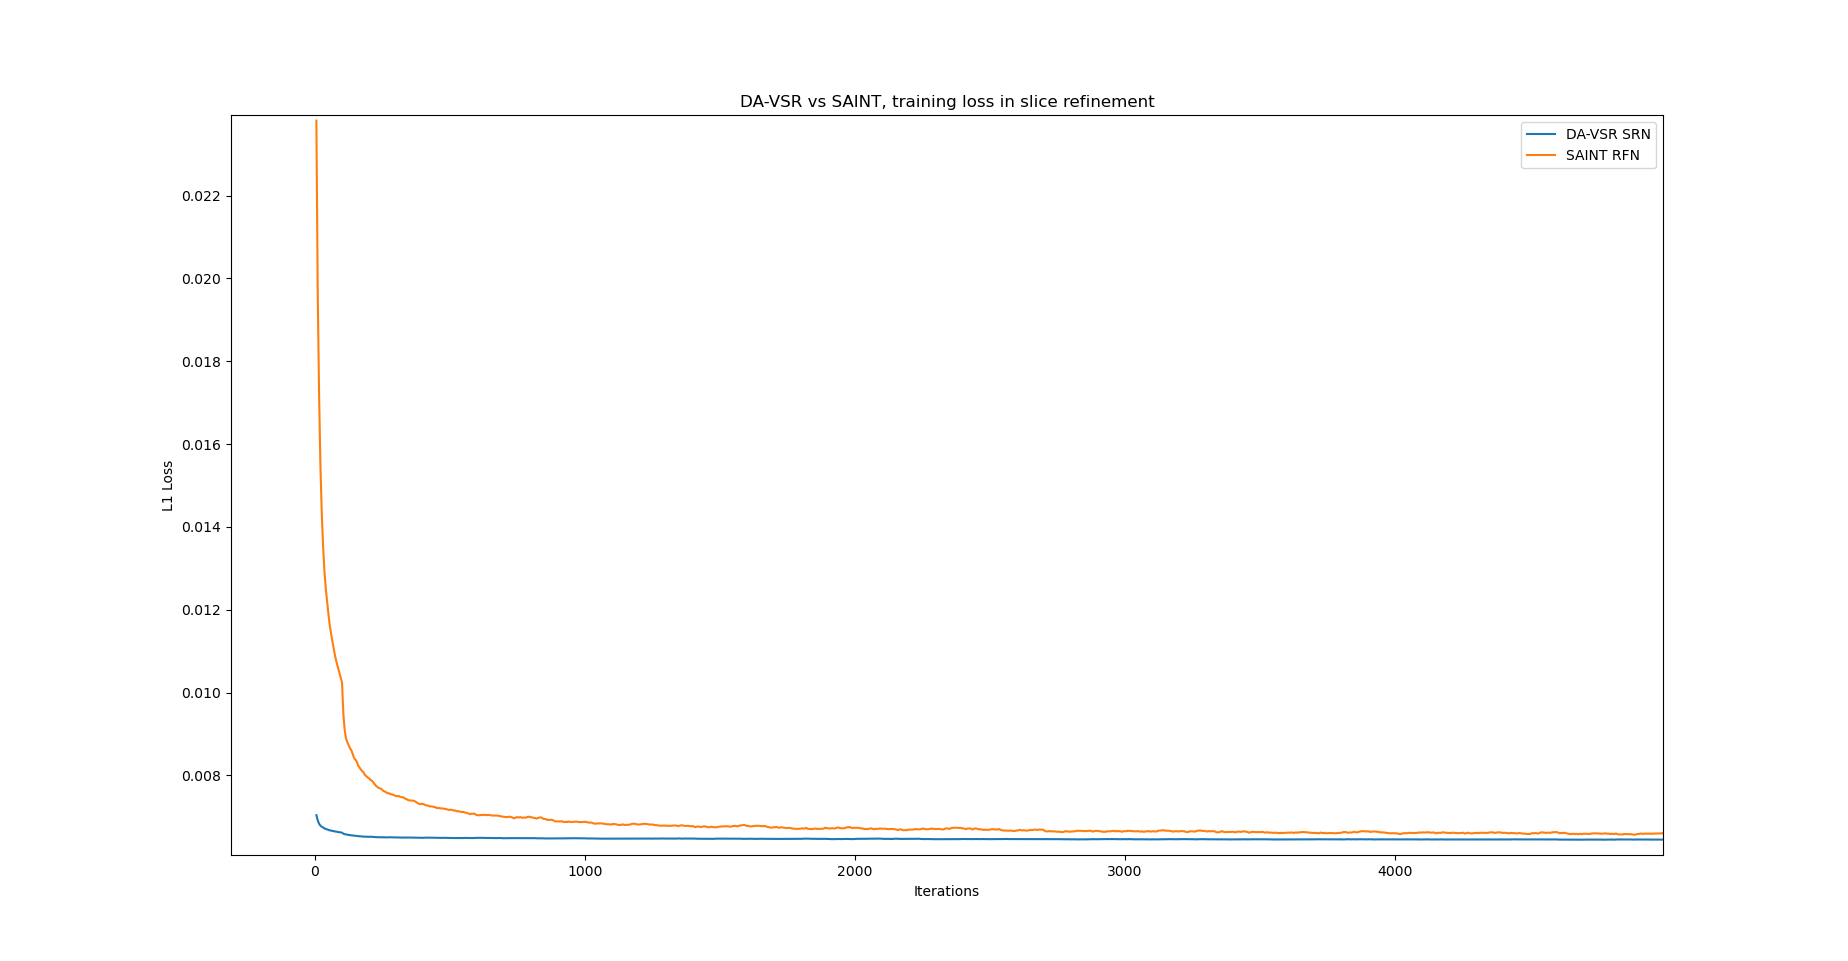}
    \caption{Comparison of DA-VSR's SRN vs SAINT's Residual-Fusion Network (RFN) in training loss. While they perform similarly after convergence, SRN converges significantly faster than RFN as it reuses features from a well-trained network. Note that RFN is five times larger than SRN in network size.}
    \label{fig:srn_converge}
\end{figure}
