# Supplementary material for: DA-VSR: Domain Adaptable Volumetric Super-Resolution For Medical Images
Source: arXiv:2210.05117 source file (2022-10-11)
Supplement: Supplementary file 3 [file img2.tex]

\begin{figure}[]
	\scriptsize
    \begin{tabular}[b]{ccc}
        \begin{subfigure}[b]{0.33\linewidth}
            \includegraphics[width=\linewidth,height=0.6\linewidth,cframe=red]{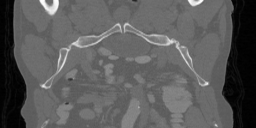}
        \caption*{Groundtruth}
        \end{subfigure}
        &
        \begin{subfigure}[b]{0.33\linewidth}
            \includegraphics[width=\linewidth,height=0.6\linewidth,cframe=red]{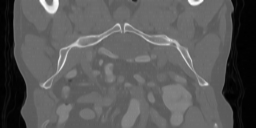}
        \caption*{$\textrm{DA-VSR}_{}$}
        \end{subfigure}
        &
        \begin{subfigure}[b]{0.33\linewidth}
            \includegraphics[width=\linewidth,height=0.6\linewidth,cframe=red]{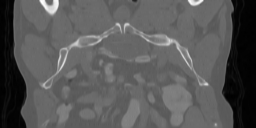}
        \caption*{$\textrm{DA-VSR}_{NA}$}
        \end{subfigure}\\
        \begin{subfigure}[b]{0.33\linewidth}
            \includegraphics[width=\linewidth,height=0.6\linewidth,cframe=red]{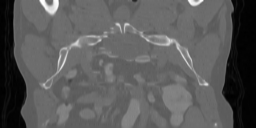}
        \caption*{SAINT}
        \end{subfigure}
        &
        \begin{subfigure}[b]{0.33\linewidth}
            \includegraphics[width=\linewidth,height=0.6\linewidth,cframe=red]{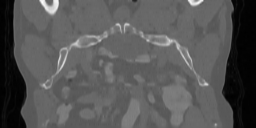}
        \caption*{3DRDN}
        \end{subfigure}
        &
        \begin{subfigure}[b]{0.33\linewidth}
            \includegraphics[width=\linewidth,height=0.6\linewidth,cframe=red]{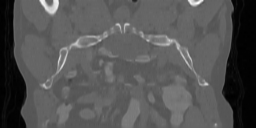}
        \caption*{3DRCAN}
        \end{subfigure}
    \end{tabular}       
    \caption{Additional visual comparisons of DA-VSR and other state-of-the-art implementations from the coronal plane.} 
    \vspace{-1em}
\end{figure}
